# Supplementary material for: An Online Probabilistic Distributed Tracing System
Source: arXiv:2405.15645 source file (2024-05-24)
Supplement: Supplementary file 1 [file appendix.tex]

\section*{Appendix}
\section{Span utility measures}
\label{sec:utilityapp}

% We study various statistical measures that can be used to measure how much utility each span contributes to performance diagnosis.
We study various ways to measure the utility of a span through performance anomaly injection experiments on widely used cloud benchmark applications (i.e., Social network, Media, and Train ticket) and 
problems include random delays and resource contentions (\cref{sec:apparatus}).
\begin{figure}[h]
\includegraphics[width=0.9\columnwidth]{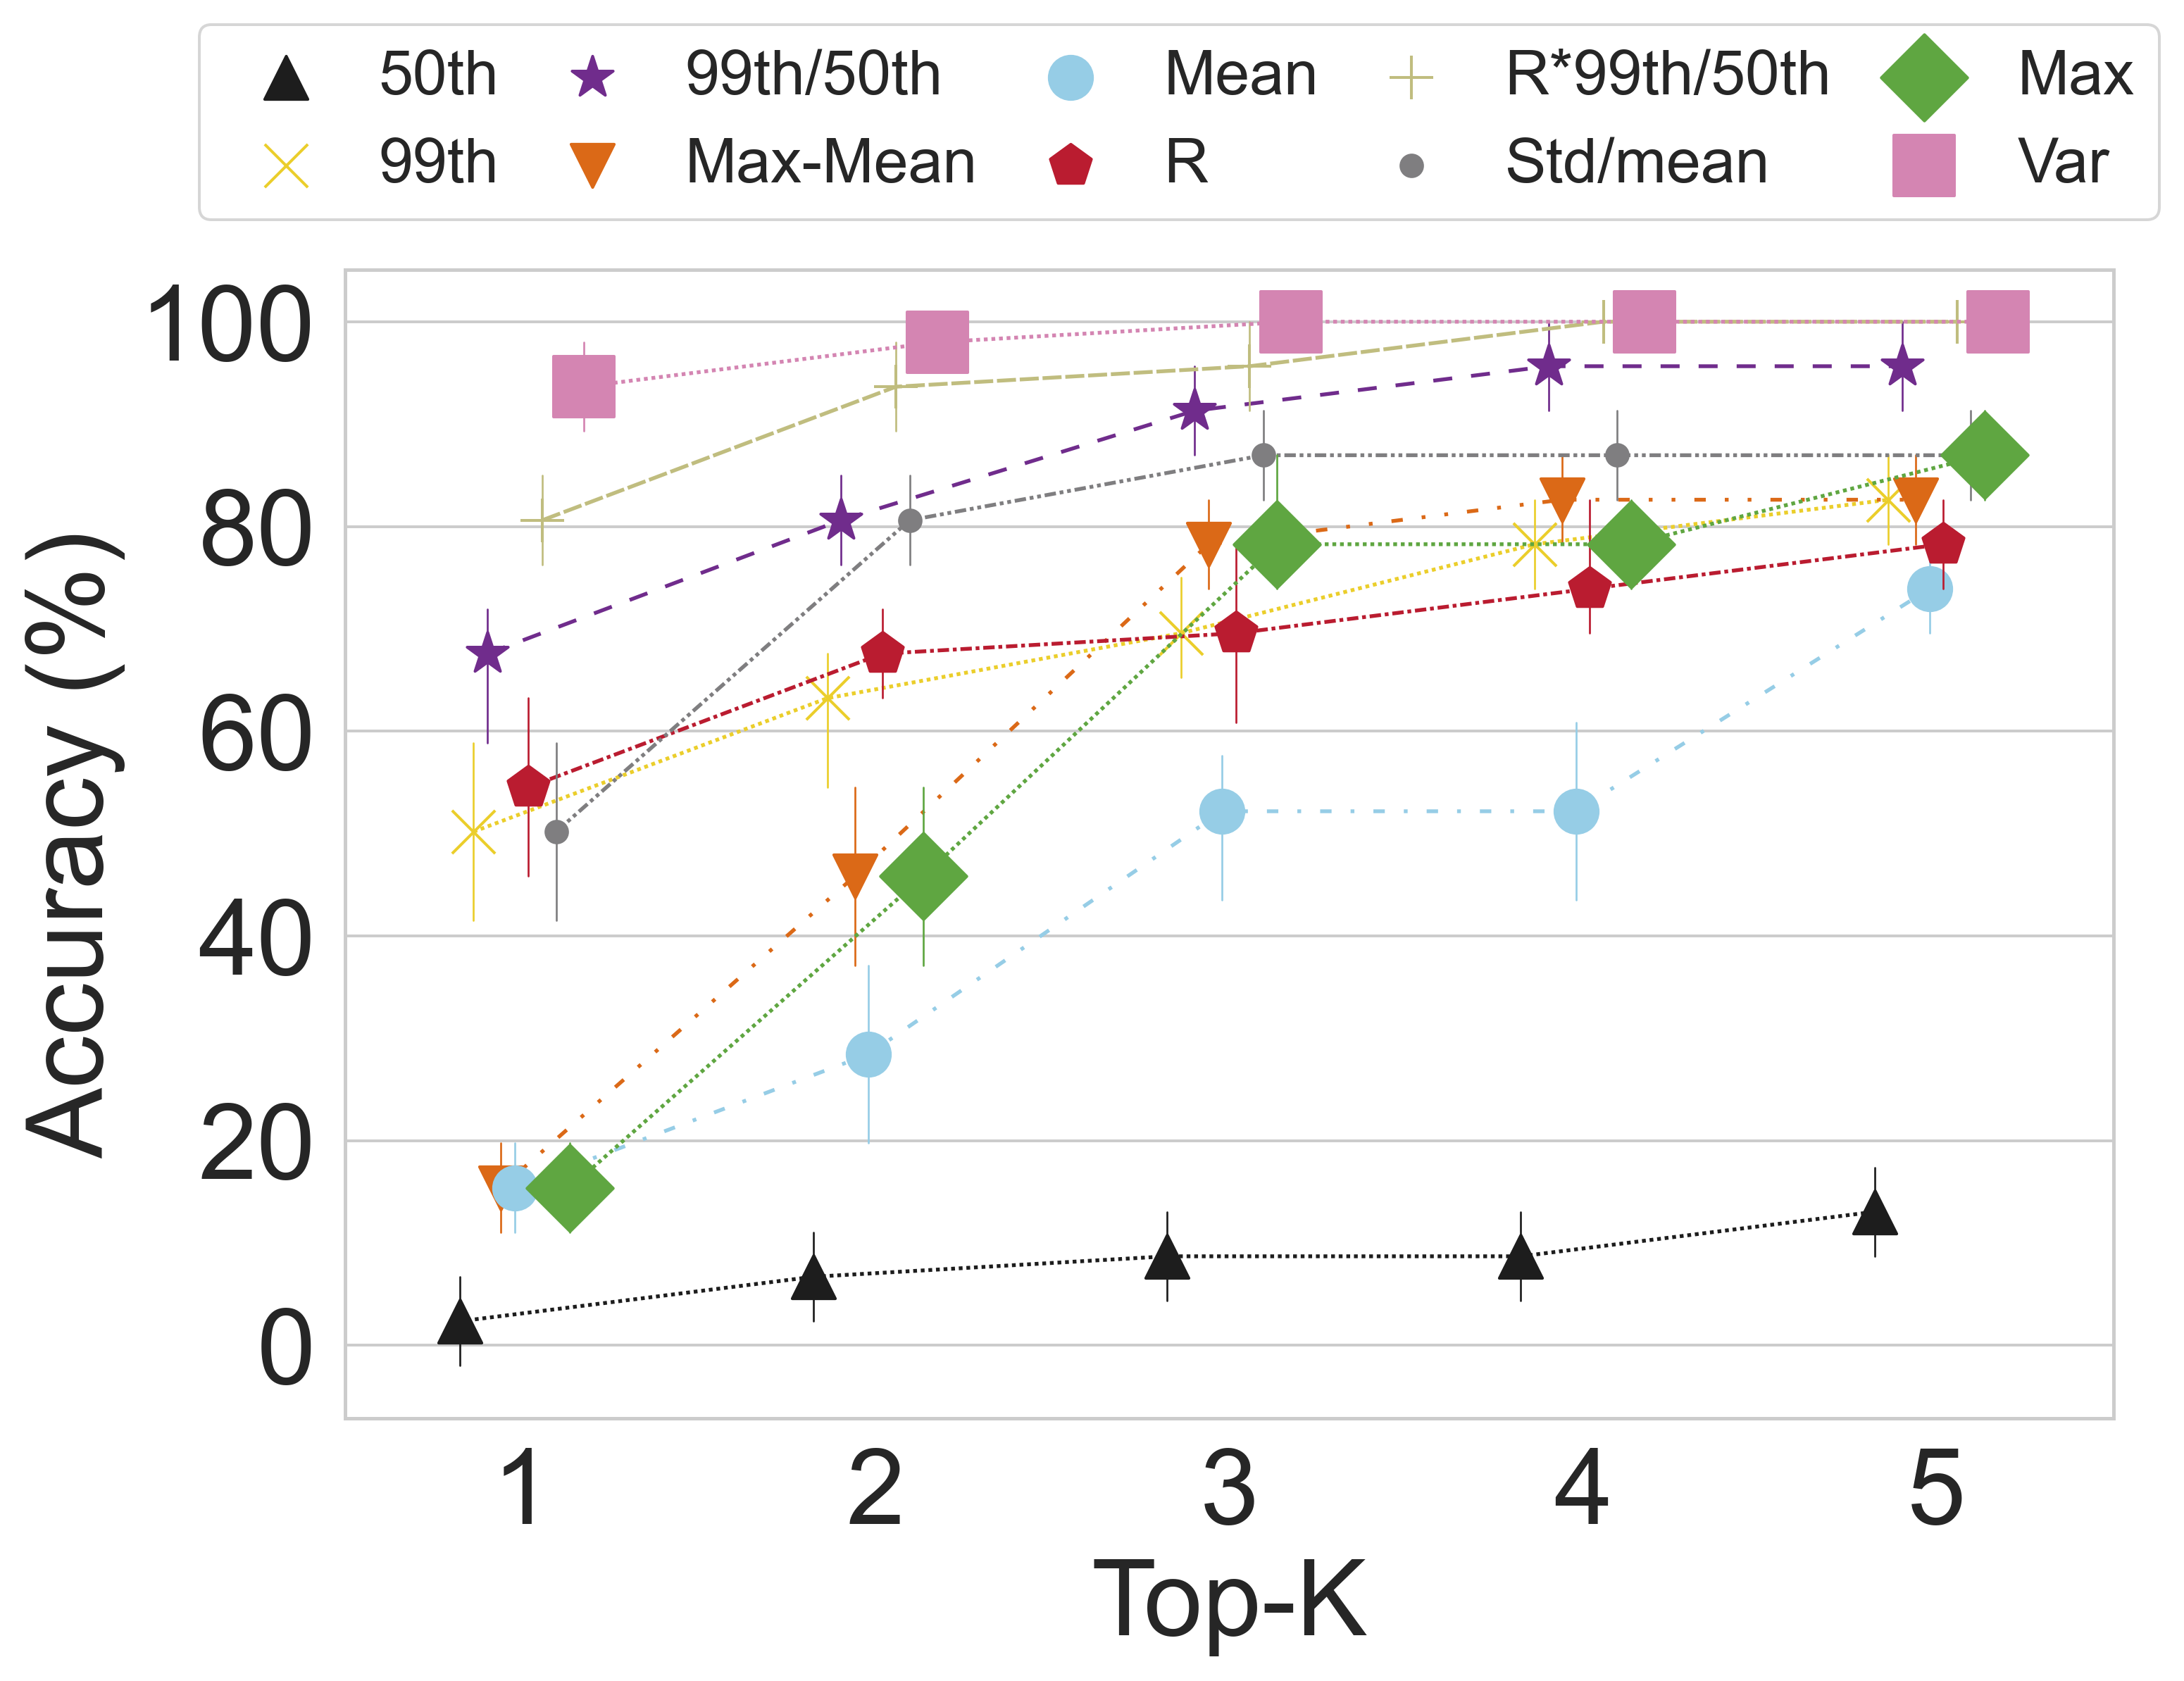}
\centering
\caption{Various statistical measures for span utilities. Figures evaluates accuracy in terms of whether top-k spans (with the maximum sampling
probabilities in Astraea with given utility) capture the faulty spans. }
\label{fig:utility}
\end{figure}
% \begin{wrapfigure}{r}{0.22\textwidth}
%  \vspace{-10pt}
%   \begin{center}
%     \includegraphics[width=\linewidth]{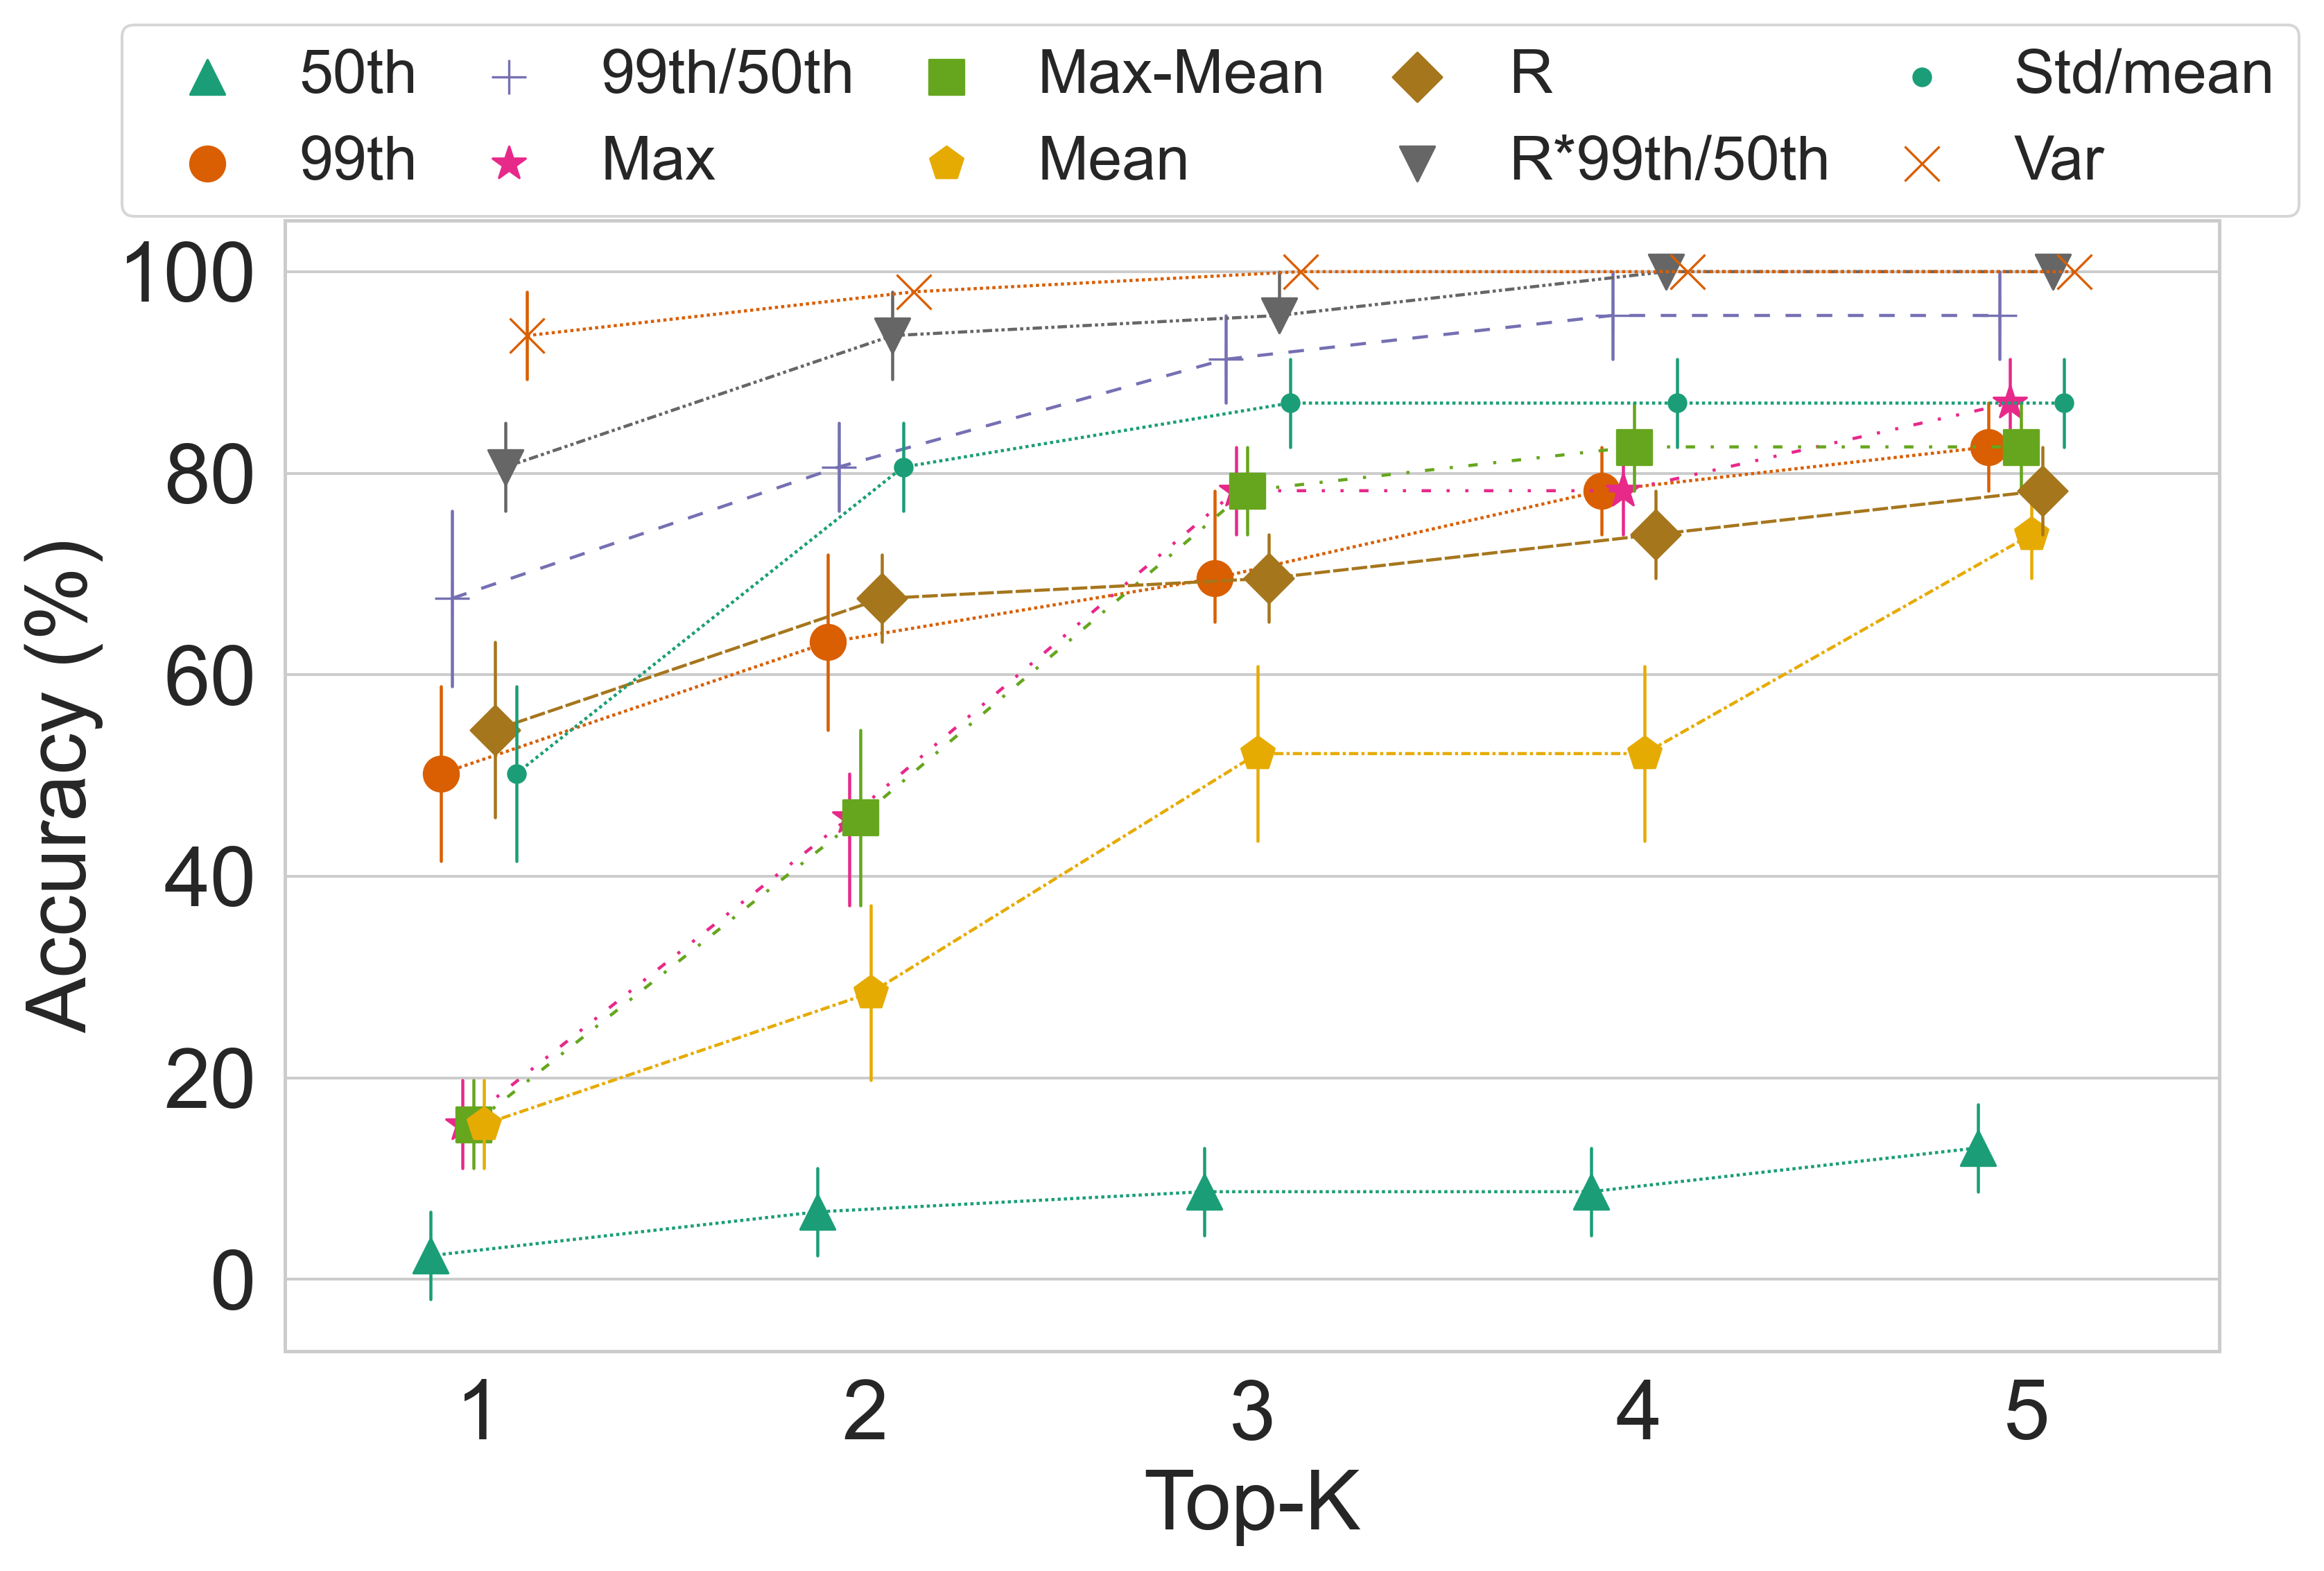}
%   \end{center}
%   \vspace{-10pt}
%   \caption{Various utility.}
%   \label{fig:utility}
%   \vspace{-10pt}
% \end{wrapfigure}
Figure \ref{fig:utility} shows the top-K accuracy (i.e., whether the correct span is among the top-K rankings) per statistical measure.
One common heuristic is to pick the span with the highest latency to detect problematic operations \cite{firm, log2}. We find that picking this measure is not ideal. Our empirical study reveals that the latency variance leads to the best results, consistent with recent research \cite{vaif,firm}, thereby the default utility in Astraea. 
Besides the out-of-the-box utility measures provided, Astraea allows developers to specify their own measures to cater to their own scenarios.

\section{Algorithm comparison}
\label{sec:algs}
Astraea embodies a novel Approximate Bayesian Sampling (ABS) algorithm, built on Bayesian learning and multi-armed bandit frameworks, to accurately eliminate extraneous instrumentation (spans) in traces. 
Action elimination algorithms such as Median elimination (ME \cite{me}) or Exponential-gap elimination (EGE \cite{ege}) also aims to find, with high probability,
optimal arms in the classical multi-armed bandit problem.
We therefore evaluate and compare ABS algorithm with the ME and EGE using production traces (\cref{sec:production}).
The figure reveals that our ABS algorithm makes elimination decisions significantly faster than baselines.
In particular, results averaged from 20 runs revealed that ABS confidently eliminates 90\% of the spans, while EGE could only halve the set, and ME could not eliminate any of them within 2000 samples.
The main advantages of our approach are that 
a) it terminates earlier than alternatives because it requires a much smaller number of samples,
b) does not require fixed sample sizes to make elimination decisions in contrast to alternatives \cite{me,ege}, and % ME and EGE %requires minimum number of samples to make elimination decisions,
c) incorporate batched updates, which is a practical necessity as traces are not available instantaneously.
\begin{figure}[h]
    \includegraphics[width=0.85\columnwidth]{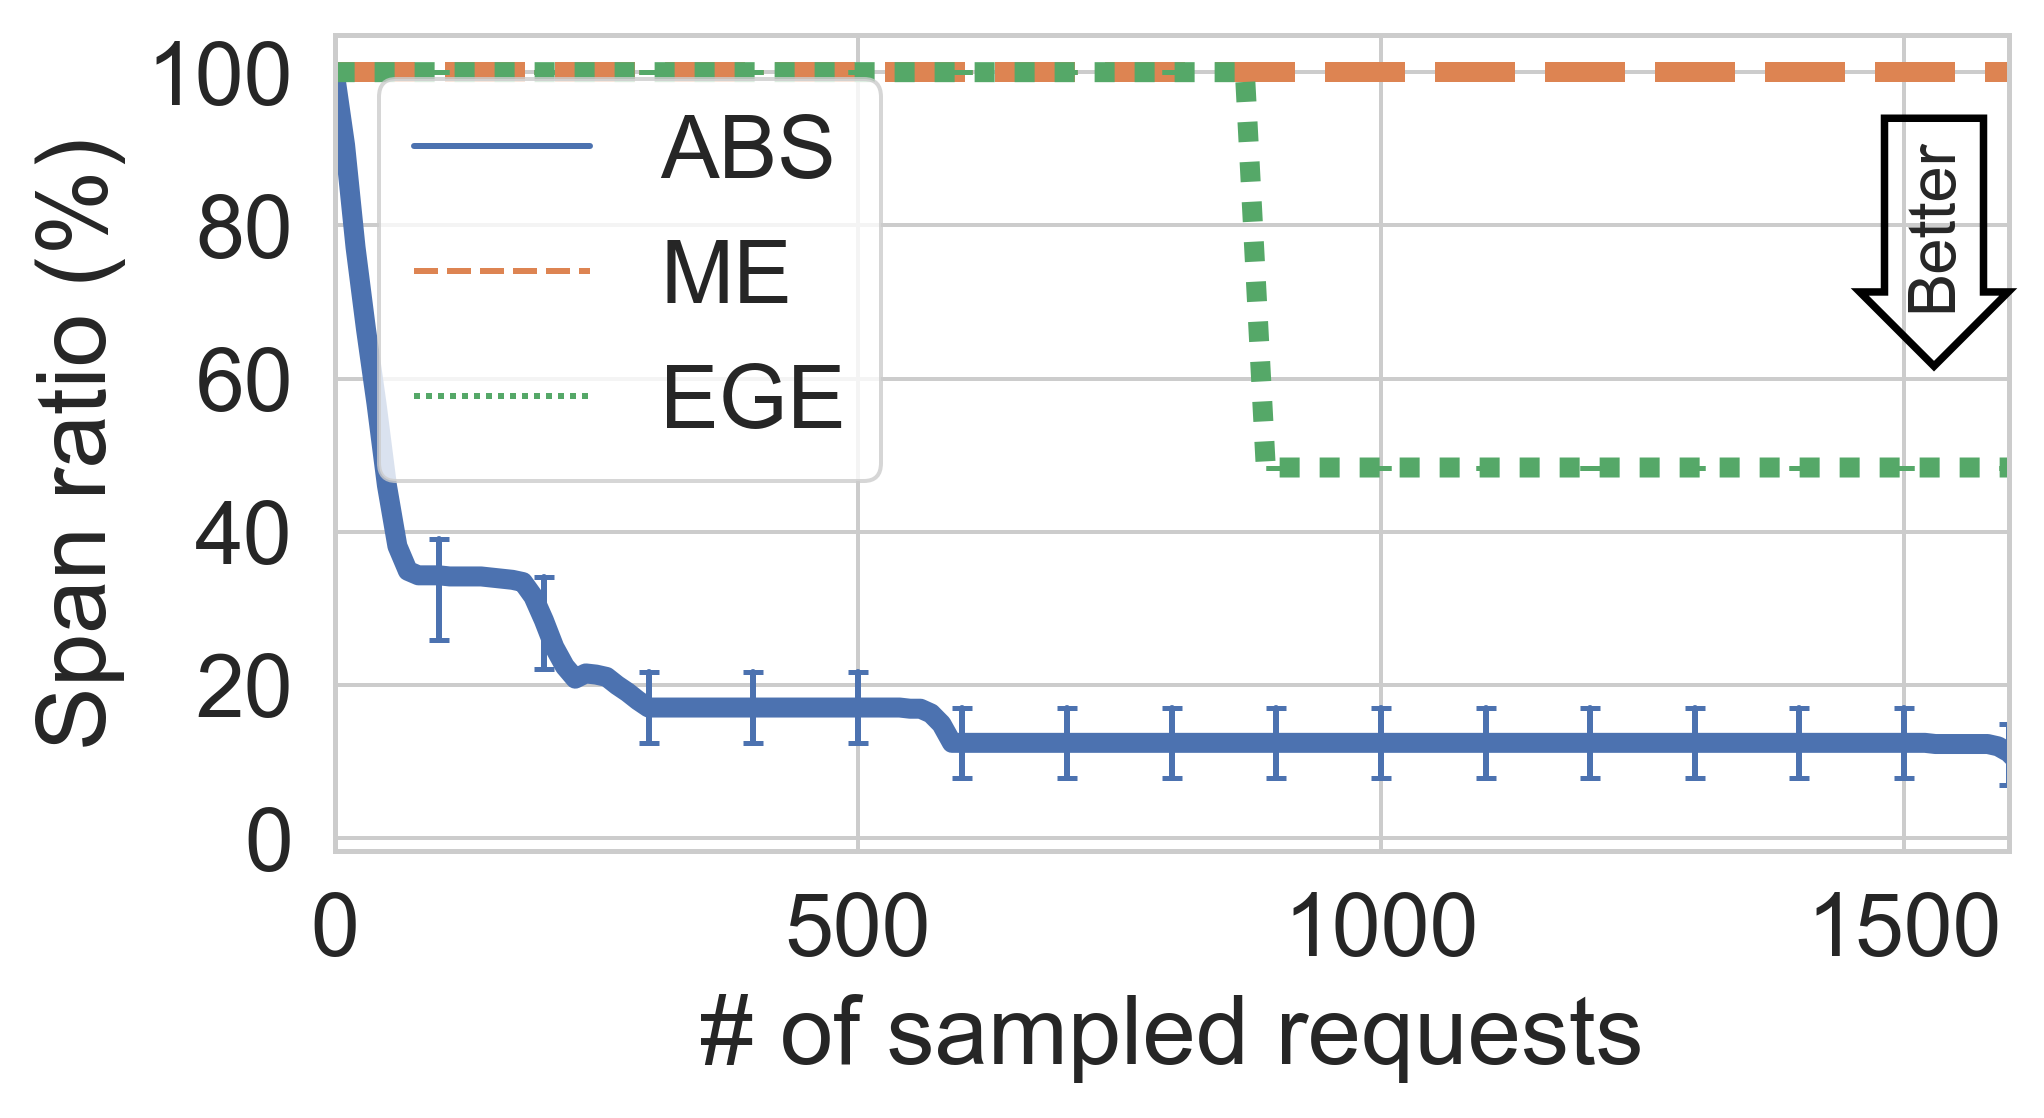}
    \centering
    \caption{Algorithm comparison. Our ABS algorithm makes elimination decisions significantly faster than baselines.}
    \label{fig:utility}
\end{figure}
